# Supplementary material for: Learning Hierarchical Control for Robust In-Hand Manipulation
Source: arXiv:1910.10985 source file (2019-10-24)
Supplement: Supplementary file 1 [file 7_appendix.tex]

\section{Design of Reinforcement Learning Controller}
\label{chpt:DRLappend}
Figure~\ref{fig:hierarchy} shows the detailed architecture of the proposed hierarchical system.
The policy network (two-fully connected layers) outputs a sequence of discrete manipulation primitives. Table~\ref{tab:ActionSpace} in the main paper lists the actions that the network can output: reposing the object $\Delta$ or $-\Delta$ in the direction of $x, y$ or $\theta$, sliding one of the fingers on the pole in either the clockwise ($+\Delta \boldsymbol{C}^i$) or anticlockwise direction($-\Delta \boldsymbol{C}^i$), or flipping a finger. Note that when choosing to flip, there are always to choices, which are flipping either the left or the right finger on the side where two fingers are currently in contact with the object. Flipping the incorrect finger will cause the object to drop. After the policy outputs one of these actions $\boldsymbol{A}$, the action is checked for feasibility using inverse kinematics. If feasible, the action will be sent to the low-level controller. The low-level controller will execute closed-loop torque control for $n$ steps to reach the temporary goal. It returns to the mid-level policy regardless of whether the temporary goal is reached or not.

    % \begin{table}[h]
    %     \centering
    %     \caption{Action space of 14 possible actions for the discrete controller in the 2D space}
    %     \makebox[\textwidth][c]
    %     {
    %         \begin{tabular}{c|c}
    %             \hline
    %              Motion Type & Parameters\\
    %             \hline
    %             Reposing & $+\Delta\boldsymbol{X}^x$, $-\Delta\boldsymbol{X}^x$, $+\Delta\boldsymbol{X}^y$, $-\Delta\boldsymbol{X}^y$, $+\Delta\boldsymbol{X}^\theta$, $-\Delta\boldsymbol{X}^\theta$  \\
    %             \hline
    %             Sliding & $+\Delta \boldsymbol{C}^1$, $-\Delta \boldsymbol{C}^1$, $+\Delta \boldsymbol{C}^2$, $-\Delta \boldsymbol{C}^2$, $+\Delta \boldsymbol{C}^3$, $-\Delta \boldsymbol{C}^3$
    %             \\
    %             \hline
    %             Flipping & Flip either left or right finger to the other side \\
    %             \hline
    %         \end{tabular}
    %     }
    %     \label{tab:ActionSpace}
    % \end{table}

    % The workflow of our architecture is shown in Figure~\ref{fig:hierarchy}: our DRL network consists of two fully connected layers. The DRL model picks one action, and the low-level controller conducts the corresponding motion primitive in a closed-loop pattern for $n$ steps.
    
    \begin{figure}[h]
        \centering
        \includegraphics[width=0.9\textwidth]{./figure/MotionPlanner.png}
        \caption{An overview of the proposed architecture. Given a state $\boldsymbol{S}_0$ and a goal pose $\boldsymbol{X}_g$, the learned policy outputs an action $\boldsymbol{A}_0$. The feasible action filter determines whether this action is valid. If yes, it generates $\boldsymbol{A}'_0$ that is sent to the low-level controller that executes closed-loop torque control for $n$ steps until the policy outputs a new action $\boldsymbol{A}_1$.} 
        \label{fig:hierarchy}
    \end{figure}

\section{Experiment Setup}

\subsection{Simulation setup} \label{append:Setup}
% \struct{Describe the manipulator to use: what's the detailed sizes, what the joints are like, what's the distance between the fingers; consider the plane is horizontal}
We evaluate the proposed approach in a simulated environment that is implemented in PyBullet~\cite{coumans2019}. The environment is 3D, but the manipulation is conducted in a horizontal 2D plane, i.e. the fingertips and object only change position within this plane. The object can additionally rotate around one axis. We do not add gravity in this simulation platform. However, we consider the object is dropped there is no contact with any finger on at least one of the sides.
%The direction of gravity is perpendicular to the working plane, and is expected to be balanced by the frictional force on the fingertips. Therefore, if there are more than two fingers lose contact with the object, we consider the object dropped.

Each finger of the hand has two joints that rotate in the plane. They have no joint limits. The width of the finger links is 2cm. The other dimensions are shown in Figure~\ref{fig:HandDimension}.

\begin{figure}
    \centering
    \includegraphics[width = 0.5\linewidth]{figure/HandDimension.png}
    \caption{Dimension of the 3-fingered hand in the experiment.}
    \label{fig:HandDimension}
\end{figure}

\subsection{Dataset}
\label{append:dataset}
% \struct{Some extra dataset information}
The overall motion range of the pole object is set to be $[-30,30]$ (cm) in $x$ direction and $[-20,20]$ (cm) in $y$ direction. Because not all the poses are reachable, we collect a dataset to train the DRL controller, which should cover the entire range of reachable object poses.
%\struct{How we sample in this state space. }
To locate the reachable range, we search all the $\boldsymbol{X}$ in the space, and use inverse kinematics to calculate whether any $\boldsymbol{C}$ can reach this state. All the  reachable $\boldsymbol{X}$s  and the corresponding $\boldsymbol{C}$s constitute the final dataset. 
The size of the dataset is given in Table~\ref{tab:dataset_info}. Figure~\ref{fig:goal_vis}(b) in the main paper shows a subset of the dataset.
We then randomly choose two reachable poses as the initial and goal pose for training, and divide them into three groups according to the difficulty to achieve the goals. The average distances between initial poses and goal poses are shown in Table~\ref{tab:GoalGroups}.

\begin{table}[h]
    \centering
    \caption{The number of contact configurations and reachable poses in the dataset}
    \makebox[\textwidth][c]
    {
        \begin{tabular}{c|ccc}
            \hline
            & $$\mathbb{F}_1$$ & $$\mathbb{F}_2$$ & $$\mathbb{F}_3$$ \\
            \hline
            Contact Configuration Number & 5649 & 3185 & 2915 \\
            Reachable Poses Number & 12303 & 5218 & 7619 \\
            \hline
        \end{tabular}
    }
    \label{tab:dataset_info}
\end{table}

 \begin{table}[h]
    \centering
    \caption{Average distances between the initial and goal poses in different data groups}
    \makebox[\textwidth][c]
    {
        \begin{tabular}{c|ccc}
            \hline
            & Easy Group & Medium Group & Hard group\\
            \hline
             Translational Distance (cm) & 6.04 & 7.02 & 8.57 \\
            Rotational Distance ($^\circ$) & 9.17 & 10.32 & 20.30 \\
            \hline
        \end{tabular}
    }
    \label{tab:GoalGroups}
\end{table}

\section{Additional Experiment Result}
In this section, we report detailed results about the basic experiment on manipulating the pole object to a goal pose, which is introduced in Section~\ref{chpt:Experiment1}. After training with each method for a comparable amount of time, we not only find considerable difference in the time it takes for our hybrid method to converge compared to these baselines (Figure~\ref{fig:LearningCurves}), we also find that our method has superior performance in all three of the goal types. Examples of the successful episodes are shown in Figure~\ref{fig:MoreExamplePPO} and Figure~\ref{fig:MoreExampleDDPG}.

% \struct{The training curve}
\begin{figure}[h!]
    \centering
    \includegraphics[width=0.95\linewidth]{figure/learningcurves.png}
    \caption{(Left) Learning curve of PPO (averaged over 5 seeds) on the in-hand object manipulation task (total 2e7 interactions with the environment). (Right) Learning curve of DDPG (averaged over 5 seeds), on the same task (total 1e7 interactions with the environment).}
    \label{fig:LearningCurves}
\end{figure}

\begin{figure}[h!]
    \centering
    \includegraphics[width=0.95\linewidth]{figure/ExampleSnapshotAppendixPPO.png}
    \caption{Snapshots of successful episodes of our method. The goal pose is indicated in red.}
    \label{fig:MoreExamplePPO}
\end{figure}

\begin{figure}[h!]
    \centering
    \includegraphics[width=0.95\linewidth]{figure/ExampleSnapshotAppendixDDPG.png}
    \caption{Snapshots of successful episodes of DDPG. The goal pose is indicated in red.}
    \label{fig:MoreExampleDDPG}
\end{figure}
